# Supplementary material for: Robust Stance Detection: Understanding Public Perceptions in Social Media
Source: arXiv:2309.15176 source file (2024-07-01)
Supplement: Supplementary file 1 [file appendix.tex]

\section{Algorithm}

\begin{algorithm}[!ht]
\small
\caption{The Learning Process of \model}
    \label{alg:learning}

	\begin{algorithmic}[1]
		\REQUIRE~~ Given $x$ = training examples, $\mathcal{D}$ = dataset, $\mathcal{S}$ = source domain, $\mathcal{T}$ = target domain, G = generator, I = number of counterfactuals, CD = contrastive data sampler, $\mathrm{F}$ = classifier model
        \FOR{$i$ < $I$}
            \FOR{$w$ in $x$}
                \STATE mask $w$ if $mask(w,\mathcal{S}, \mathcal{T}) > \tau $
            \ENDFOR
            \FOR{$M(x)$}
                \STATE $x' = G(M(x), v')$
            \ENDFOR
        \ENDFOR
        \STATE $\mathcal{D}_{total}$ = CD$(x', x)$
        \FOR{batch $b \in \mathcal{D}_{total}$}
            \STATE $\ell_{CE}, \ell_{cont} = \mathrm{F}(b)$
            \STATE $\ell_{total} = \lambda \ell_{\mathrm{cont}} + (1 - \lambda) \ell_{\mathrm{CE}}$
            \STATE update $\mathrm{F}$ based on $\ell_{total}$
        \ENDFOR
	\end{algorithmic}
	
\end{algorithm}

\newpage
\section{Examples of the Generated Counterfactuals}

\begin{table}[!ht] 
\scriptsize
\begin{center}
    \caption{In this table, CoVaxNet\_pre was solely used as the source domain to generate counterfactuals toward the following target domains. During training, 30\% were randomly selected from each target domain.}
    % \label{tab:table1}
    \begin{tabular}
    {p{0.13\linewidth}|p{0.36\linewidth}|p{0.36\linewidth}}
        \toprule % <-- Toprule here
        \textbf{Target Domain} & \textbf{Source Example} & \textbf{Target Example}\\
        \midrule
        CoVaxNet \_post & These days \textcolor{blue}{can} happen again, but we have to want them badly enough to MAKE them happen again... & These days \textcolor{blue}{we want them to} happen again, but we have to want them badly enough to MAKE them happen again...\\
        
        \midrule % <-- Midrule here
        Wearing face masks  & The choice of taking the \textcolor{blue}{vaccine} or not should be the decision of the individual... & The choice of taking the \textcolor{blue}{mask} or not should be the decision of the individual... \\
        
        \midrule % <-- Midrule here
        Keeping schools closed &  I would really like for \textcolor{blue}{people} to read what HIPPA actually says before they start using it as a rebuttal against disclosing vaccination status... & I would really like for \textcolor{blue}{schools} to read what HIPPA actually says before they start using it as a rebuttal against disclosing vaccination status... \\
        
       \midrule % <-- Midrule here
        Stay-at-home orders & Thank you We need everyone to \textcolor{blue}{get immunized}!!!! & Thank you We need everyone to \textcolor{blue}{stay inside}!!!! \\
      \bottomrule % <-- Bottomrule here
    \end{tabular}
  \end{center}
\end{table}

% \section{Parameter Analysis on Cross-Domain Experiments}
% \begin{table*}[ht]
%   \begin{center}
%     \caption{Parameter Analysis on Cross-Domain Experiments}
%     \label{tab:parameter}
%     \begin{tabular}{l|l|l|l|l|l|l|l|l}
%       \toprule % <-- Toprule here
%       \textbf{Method} & \multicolumn{4}{c|}{\textbf{Accuracy}} & \multicolumn{4}{c}{\textbf{MacroF1}}\\ 
%        & $\gamma=0.05$ & $0.15$ & $0.3$ & $0.45$ & $0.05$ & $0.15$ & $0.3$ & $0.45$ \\
%       \midrule % <-- Midrule here
%       BERT base & 0.674 & 0.707 & 0.750 & - & 0.749 & 0.751 & 0.786 & -\\
%       \midrule % <-- Midrule here
%       MoLE & 0.80 &	0.72 &	0.80 &	0.77 &	0.89 &	0.58&	0.82  & 0.67 \\
%       MTL w/ BERTBase   & 0.80 &	0.72 &	0.80 &	0.77 &	0.89 &	0.58 &	0.82 &	0.69\\
%       RLFND & 0.85 &	0.68 &	0.79 &	0.88 &	0.62 &	0.74 &	0.93 & - \\
%       \midrule % <-- Midrule here
%       \model & 0.679 & 0.716 & 0.721 & 0.772 & 0.728 & 0.761 & 0.762 & 0.817 \\
%       \model~w/ source dataset & 0.698 & 0.746 & 0.767 & 0.781 & 0.767 & 0.783 & 0.809 & 0.818 \\
%       \bottomrule % <-- Bottomrule here
%     \end{tabular}
%   \end{center}
% \end{table*}
